# Supplementary material for: Accurate atomic quantum defects from particle-particle random phase approximation
Source: arXiv:1510.07579 source file (2015-10-26)
Supplement: Supplementary file 1 [file Suppl_material_for_online_version.pdf]

I. Excitation Data

Be

| Configuration | Term | Expt | TDAHF |
|---|---|---|---|
| 1s22s3d | 1D | 0.293571922 | 0.29378556 |
| 1s22s4d | 1D | 0.313404594 | 0.31305813 |
| 1s22s5d | 1D | 0.323526939 | 0.3228695 |
| 1s22s6d | 1D | 0.329217751 | 0.32842134 |
| 1s22s2p | 1P | 0.193951856 | 0.19595018 |
| 1s22s3p | 1P | 0.274247666 | 0.27372815 |
| 1s22s4p | 1P | 0.305448107 | 0.30467293 |
| 1s22s5p | 1P | 0.31950871 | 0.31857456 |
| 1s22s3s | 1S | 0.24914061 | 0.24815038 |
| 1s22s4s | 1S | 0.297294708 | 0.2962544 |
| 1s22s5s | 1S | 0.315871261 | 0.31481834 |
| 1s22s6s | 1S | 0.324979603 | 0.32392142 |
| 1s22s3d | 3D | 0.282751929 | 0.28326146 |
| 1s22s4d | 3D | 0.309580742 | 0.30908456 |
| 1s22s5d | 3D | 0.321710768 | 0.32091798 |
| 1s22s6d | 3D | 0.32820724 | 0.32729641 |
| 1s22s2p | 3P | 0.100145498 | 0.10046467 |
| 1s22s3p | 3P | 0.268415766 | 0.26759982 |
| 1s22s4p | 3P | 0.304432819 | 0.30345929 |
| 1s22s5p | 3P | 0.319257699 | 0.3182374 |
| 1s22s3s | 3S | 0.23731029 | 0.23648002 |
| 1s22s4s | 3S | 0.293927968 | 0.29293659 |
| 1s22s5s | 3S | 0.314449614 | 0.31341572 |
| 1s22s6s | 3S | 0.324247666 | 0.32319767 |

Mg

| Configuration | Term | Expt | TDAHF |
|---|---|---|---|
| 3s3d | 1D | 0.211438681 | 0.20602693 |
| 3s4d | 1D | 0.242111562 | 0.23628246 |
| 3s5d | 1D | 0.256572918 | 0.25111231 |
| 3s6d | 1D | 0.264386814 | 0.25910715 |
| 3s3p | 1P | 0.159713436 | 0.15678475 |
| 3s4p | 1P | 0.224851683 | 0.22013825 |
| 3s5p | 1P | 0.249274002 | 0.24424541 |
| 3s6p | 1P | 0.260703951 | 0.25559855 |
| 3s4s | 1S | 0.198225854 | 0.19370097 |
| 3s5s | 1S | 0.23947588 | 0.23453168 |
| 3s6s | 1S | 0.256019258 | 0.25094924 |
| 3s7s | 1S | 0.264323778 | 0.25920252 |
| 3s3d | 3D | 0.218519412 | 0.21555002 |
| 3s4d | 3D | 0.24693065 | 0.24251772 |
| 3s5d | 3D | 0.259579508 | 0.2547618 |
| 3s6d | 3D | 0.266298699 | 0.2613211 |
| 3s3p | 3P | 0.099562837 | 0.09442203 |

| | | | |
|---|---|---|---|
| 3s4p | 3P | 0.217991268 | 0.21297203 |
| 3s5p | 3P | 0.247188339 | 0.24208225 |
| 3s6p | 3P | 0.259802143 | 0.25466537 |
| 3s4s | 3S | 0.187718732 | 0.18342316 |
| 3s5s | 3S | 0.236360647 | 0.23148505 |
| 3s6s | 3S | 0.254674752 | 0.24963363 |
| 3s7s | 3S | 0.263621165 | 0.25851446 |

Li

| Configuration | Term | Expt | TDAHF(AB) | TDAHF(BB) | TDAHF(average) |
|---|---|---|---|---|---|
| 1s23d | 2D | 0.14254344 | 0.14677314 | 0.13931706 | 0.1430451 |
| 1s24d | 2D | 0.166876883 | 0.17108706 | 0.16363166 | 0.16735936 |
| 1s25d | 2D | 0.178138662 | 0.1823451 | 0.1748901 | 0.1786176 |
| 1s26d | 2D | 0.184255311 | 0.18864641 | 0.18119153 | 0.18491897 |
| 1s22p | 2P | 0.067909519 | 0.07398197 | 0.06546026 | 0.069721115 |
| 1s23p | 2P | 0.140913561 | 0.14568582 | 0.13789622 | 0.14179102 |
| 1s24p | 2P | 0.166175965 | 0.17061638 | 0.16301905 | 0.166817715 |
| 1s25p | 2P | 0.177777031 | 0.18211653 | 0.17458831 | 0.17835242 |
| 1s23s | 2S | 0.12396652 | 0.12722886 | 0.12144748 | 0.12433817 |
| 1s24s | 2S | 0.159534803 | 0.16338122 | 0.15655204 | 0.15996663 |
| 1s25s | 2S | 0.174514259 | 0.17854162 | 0.17138604 | 0.17496383 |
| 1s26s | 2S | 0.182206358 | 0.18630968 | 0.17902116 | 0.18266542 |

II. Fit results that obtain IP

Expt for Be and Mg

| | | IP | a | b | c |
|---|---|---|---|---|---|
| Be | s1 | 0.342614 | 0.673422 | -0.081206 | 0.735512 |
| | s3 | 0.342627 | 0.777386 | -0.332850 | 0.978906 |
| | p1 | 0.342595 | 0.369442 | 0.993130 | -0.472750 |
| | p3 | 0.342676 | 0.375213 | -0.048087 | 5.013414 |
| | d1 | 0.342597 | -0.103480 | 0.416170 | -25.383600 |
| | d3 | 0.342635 | 0.114736 | 0.182650 | 1.859927 |
| Mg | s1 | 0.280989 | 1.519738 | -0.189129 | 1.047760 |
| | s3 | 0.281019 | 1.631339 | -0.427148 | 1.967129 |
| | p1 | 0.280991 | 1.046403 | 0.496601 | -0.686030 |
| | p3 | 0.281046 | 1.140627 | -0.220250 | 8.017493 |
| | d1 | 0.280960 | 0.584536 | 4.919181 | 21.134803 |
| | d3 | 0.281011 | 0.171078 | 0.092490 | 1.555441 |

ppTDAHF for Be and Mg

| | | IP | a | b | c |
|---|---|---|---|---|---|
| Be | s1 | 0.341546 | 0.671971 | -0.088525 | 0.716513 |
| | s3 | 0.341550 | 0.773313 | -0.372564 | 0.753695 |
| | p1 | 0.341430 | 0.338331 | 0.620530 | -2.435130 |
| | p3 | 0.341601 | 0.369662 | -0.064905 | 5.034753 |
| | d1 | 0.341645 | -0.123940 | 1.801410 | -6.081700 |

| | | | | | |
|---|---|---|---|---|---|
| | d3 | 0.341565 | 0.083503 | 0.231680 | 0.499370 |
| Mg | s1 | 0.275822 | 1.512380 | -0.125650 | 1.526208 |
| | s3 | 0.275820 | 1.614787 | -0.565840 | 1.200163 |
| | p1 | 0.275846 | 1.045046 | 0.710559 | -0.079670 |
| | p3 | 0.275892 | 1.139445 | -0.160949 | 8.503502 |
| | d1 | 0.275864 | 0.605478 | 4.128028 | 10.361063 |
| | d3 | 0.275833 | 0.133721 | 0.240405 | 0.257716 |

For Li

| | Expt<br>IP | a | b | c |
|---|---|---|---|---|
| S | 0.198152137 | 0.399489082 | -0.056306156 | 0.039764813 |
| P | 0.198152305 | 0.047266105 | 0.049086236 | -0.006848432 |
| D | 0.198149295 | -0.99921753 | -0.033301498 | -0.406046043 |

| | ppTDAHF-ab<br>IP | a | b | c |
|---|---|---|---|---|
| S | 0.202344786 | 0.415344363 | -0.06145505 | 0.01078272 |
| P | 0.202378606 | 0.035863594 | 0.120623623 | 0.384019085 |
| D | 0.202371501 | -0.9921148 | 0.259770874 | 2.51518009 |

| | ppTDAHF-bb<br>IP | a | b | c |
|---|---|---|---|---|
| S | 0.194890348 | 0.386365258 | -0.059391892 | 0.013220425 |
| P | 0.19492279 | 0.044722979 | 0.120495616 | 0.342365108 |
| D | 0.194917049 | -0.992029969 | 0.260635851 | 2.517594969 |

| | ppTDAHF-Ave<br>IP | a | b | c |
|---|---|---|---|---|
| S | 0.198617598 | 0.400894276 | -0.061903406 | 0.007610546 |
| P | 0.198650704 | 0.040297794 | 0.12043882 | 0.362565533 |
| D | 0.198644268 | -0.992074423 | 0.260134379 | 2.515783618 |

III. IP's and QD's datapoint for plot

Be 1s

| Expt-TrueIP | | Expt-FitIP | | ppTDAHF | |
|---|---|---|---|---|---|
| Exci-IP | Recal QD | Exci-IP | Recal QD | Exci-IP | Recal QD |
| -0.09346269 | 0.687052026 | -0.093473116 | 0.687181025 | -0.093395968 | 0.686225989 |
| -0.045308592 | 0.678037557 | -0.045319018 | 0.678419706 | -0.045291948 | 0.677427221 |
| -0.026732039 | 0.67517085 | -0.026742466 | 0.676013997 | -0.026728008 | 0.674844692 |
| -0.017623697 | 0.673566681 | -0.017634123 | 0.675141536 | -0.017624928 | 0.673752691 |

Be 3s

| Expt-TrueIP | | Expt-FitIP | | ppTDAHF | |
|---|---|---|---|---|---|
| Exci-IP | Recal QD | Exci-IP | Recal QD | Exci-IP | Recal QD |
| -0.10529301 | 0.8208595 | -0.105316273 | 0.82110019 | -0.105070057 | 0.818548716 |

| | | | | | |
|---|---|---|---|---|---|
| -0.048675332 | 0.794981509 | -0.048698596 | 0.795747124 | -0.048613487 | 0.79294346 |
| -0.028153686 | 0.785778371 | -0.028176949 | 0.787518403 | -0.028134357 | 0.78433097 |
| -0.018355634 | 0.780843605 | -0.018378897 | 0.784147777 | -0.018352407 | 0.780384773 |

Be 1p

| Expt-TrueIP | | Expt-FitIP | | ppTDAHF | |
|---|---|---|---|---|---|
| Exci-IP | Recal QD | Exci-IP | Recal QD | Exci-IP | Recal QD |
| -0.148651444 | 0.165995335 | -0.148642735 | 0.165941607 | -0.145479927 | 0.146112122 |
| -0.068355634 | 0.295432374 | -0.068346924 | 0.295260062 | -0.067701957 | 0.282407156 |
| -0.037155193 | 0.331612176 | -0.037146483 | 0.331182162 | -0.036757177 | 0.311804562 |
| -0.02309459 | 0.347034052 | -0.023085881 | 0.34615646 | -0.022855547 | 0.322765002 |

Be 3p

| Expt-TrueIP | | Expt-FitIP | | ppTDAHF | |
|---|---|---|---|---|---|
| Exci-IP | Recal QD | Exci-IP | Recal QD | Exci-IP | Recal QD |
| -0.242457802 | 0.563958733 | -0.242530487 | 0.564173935 | -0.241136477 | 0.560029663 |
| -0.074187534 | 0.40391125 | -0.074260218 | 0.405182066 | -0.074001327 | 0.400647089 |
| -0.038170481 | 0.380728318 | -0.038243166 | 0.384169338 | -0.038141857 | 0.379370522 |
| -0.023345601 | 0.372115876 | -0.023418285 | 0.37930338 | -0.023363747 | 0.373913482 |

Be 1d

| Expt-TrueIP | | Expt-FitIP | | ppTDAHF | |
|---|---|---|---|---|---|
| Exci-IP | Recal QD | Exci-IP | Recal QD | Exci-IP | Recal QD |
| -0.049031378 | -0.19336053 | -0.049025459 | -0.193553306 | -0.047859554 | -0.232218257 |
| -0.029198706 | -0.138121127 | -0.029192787 | -0.138540641 | -0.028586984 | -0.182161827 |
| -0.019076361 | -0.119614161 | -0.019070442 | -0.120408642 | -0.018775614 | -0.160454215 |
| -0.013385549 | -0.111768633 | -0.01337963 | -0.113120442 | -0.013223774 | -0.149039667 |

Be 3d

| Expt-TrueIP | | Expt-FitIP | | ppTDAHF | |
|---|---|---|---|---|---|
| Exci-IP | Recal QD | Exci-IP | Recal QD | Exci-IP | Recal QD |
| -0.059851371 | 0.109666529 | -0.059882751 | 0.110423947 | -0.058303169 | 0.071542524 |
| -0.033022558 | 0.108834983 | -0.033053938 | 0.110682516 | -0.032480069 | 0.076474033 |
| -0.020892532 | 0.107966018 | -0.020923913 | 0.111635815 | -0.020646649 | 0.078922372 |
| -0.01439606 | 0.106637193 | -0.014427441 | 0.113049922 | -0.014268219 | 0.080294243 |

Mg 1s

| Expt-TrueIP | | Expt-FitIP | | ppTDAHF | |
|---|---|---|---|---|---|
| Exci-IP | Recal QD | Exci-IP | Recal QD | Exci-IP | Recal QD |
| -0.082768146 | 1.542161234 | -0.082777146 | 1.542294853 | -0.08214503 | 1.532856811 |
| -0.04151812 | 1.529706848 | -0.04152712 | 1.530082919 | -0.04131432 | 1.521158056 |
| -0.024974742 | 1.525603221 | -0.024983742 | 1.526409209 | -0.02489676 | 1.51860128 |
| -0.016670222 | 1.523358529 | -0.016679222 | 1.524836308 | -0.01664348 | 1.518960487 |

Mg 3s

| Expt-TrueIP | | Expt-FitIP | | ppTDAHF | |
|---|---|---|---|---|---|
| Exci-IP | Recal QD | Exci-IP | Recal QD | Exci-IP | Recal QD |
| -0.093275268 | 1.684729439 | -0.093284268 | 1.68484113 | -0.09242284 | 1.674076924 |

| | | | | | |
|---|---|---|---|---|---|
| -0.044633353 | 1.653003606 | -0.044642353 | 1.653341004 | -0.04436095 | 1.642743038 |
| -0.026319248 | 1.641387466 | -0.026328248 | 1.6421325 | -0.02621237 | 1.632510623 |
| -0.017372835 | 1.635247944 | -0.017381835 | 1.63663701 | -0.01733154 | 1.628860584 |

Mg 1p

| Expt-TrueIP | | Expt-FitIP | | ppTDAHF | |
|---|---|---|---|---|---|
| Exci-IP | Recal QD | Exci-IP | Recal QD | Exci-IP | Recal QD |
| -0.121280564 | 0.969563562 | -0.121289564 | 0.969638895 | -0.11906125 | 0.950727164 |
| -0.056142317 | 1.015718155 | -0.056151317 | 1.015957326 | -0.05570775 | 1.004100826 |
| -0.031719998 | 1.029744757 | -0.031728998 | 1.030307883 | -0.03160059 | 1.022250713 |
| -0.020290049 | 1.035866509 | -0.020299049 | 1.036967107 | -0.02024745 | 1.030647155 |

Mg 3p

| Expt-TrueIP | | Expt-FitIP | | ppTDAHF | |
|---|---|---|---|---|---|
| Exci-IP | Recal QD | Exci-IP | Recal QD | Exci-IP | Recal QD |
| -0.181431163 | 1.339919837 | -0.181440163 | 1.33996101 | -0.18142397 | 1.339886929 |
| -0.063002732 | 1.182880234 | -0.063011732 | 1.183081427 | -0.06287397 | 1.179997064 |
| -0.033805661 | 1.154168209 | -0.033814661 | 1.15468004 | -0.03376375 | 1.151782022 |
| -0.021191857 | 1.142637779 | -0.021200857 | 1.143668891 | -0.02118063 | 1.141350557 |

Mg 1d

| Expt-TrueIP | | Expt-FitIP | | ppTDAHF | |
|---|---|---|---|---|---|
| Exci-IP | Recal QD | Exci-IP | Recal QD | Exci-IP | Recal QD |
| -0.069555319 | 0.318857928 | -0.069564319 | 0.319031372 | -0.06981907 | 0.323926901 |
| -0.038882438 | 0.414016742 | -0.038891438 | 0.414431688 | -0.03956354 | 0.445017802 |
| -0.024421082 | 0.475167037 | -0.024430082 | 0.476000584 | -0.02473369 | 0.503852548 |
| -0.016607186 | 0.51297457 | -0.016616186 | 0.514460769 | -0.01673885 | 0.534596968 |

Mg 3d

| Expt-TrueIP | | Expt-FitIP | | ppTDAHF | |
|---|---|---|---|---|---|
| Exci-IP | Recal QD | Exci-IP | Recal QD | Exci-IP | Recal QD |
| -0.062474588 | 0.170997692 | -0.062483588 | 0.171201441 | -0.06029598 | 0.120342591 |
| -0.03406335 | 0.168742634 | -0.03407235 | 0.169248669 | -0.03332828 | 0.126723048 |
| -0.021414492 | 0.167953452 | -0.021423492 | 0.168968529 | -0.0210842 | 0.130252553 |
| -0.014695301 | 0.166949193 | -0.014704301 | 0.168734571 | -0.0145249 | 0.132833315 |

Li s

| Expt-TrueIP | | Expt-FitIP | | ppTDAHF-ab | | ppTDAHF-bb | | ppTDAHF-ave | |
|---|---|---|---|---|---|---|---|---|---|
| Exci-IP | Recal QD | Exci-IP | Recal QD | Exci-IP | Recal QD | Exci-IP | Recal QD | Exci-IP | Recal QD |
| -0.07417548 | 0.403700328 | -0.074184726 | 0.403862124 | -0.075136104 | 0.420350717 | -0.073462582 | 0.391133193 | -0.074299354 | 0.405865531 |
| -0.038607197 | 0.401256707 | -0.038616442 | 0.40168755 | -0.038983744 | 0.41867918 | -0.038358022 | 0.38958688 | -0.038670894 | 0.404221775 |
| -0.023627741 | 0.399829743 | -0.023636986 | 0.400729528 | -0.023823344 | 0.418753725 | -0.023524032 | 0.389700718 | -0.023673699 | 0.404297101 |
| -0.015935642 | 0.398553153 | -0.015944888 | 0.400177415 | -0.016057464 | 0.419841691 | -0.015891582 | | | |

| | | |
|---|---|---|
| 0.390793457 | -0.015974534 | 0.405375947 |

Li p

| Expt-TrueIP | | Expt-FitIP | | ppTDAHF-ab | | ppTDAHF-bb | | ppTDAHF-ave | |
|---|---|---|---|---|---|---|---|---|---|
| Exci-IP | Recal QD | Exci-IP | Recal QD | Exci-IP | Recal QD | Exci-IP | Recal QD | Exci-IP | Recal QD |
| -0.130232481 | 0.040589891 | -0.130241727 | 0.040659441 | -0.128382994 | 0.026526714 | -0.129449802 | 0.034675327 | -0.128916409 | 0.030613743 |
| -0.057228439 | 0.044172721 | -0.057237685 | 0.044411463 | -0.056679144 | 0.029884352 | -0.057013842 | 0.038615171 | -0.056846504 | 0.03425967 |
| -0.031966035 | 0.045053482 | -0.031975281 | 0.045625319 | -0.031749064 | 0.03156257 | -0.031891462 | 0.040432182 | -0.031820274 | 0.036005464 |
| -0.020364969 | 0.045006145 | -0.020374215 | 0.046130559 | -0.020257684 | 0.031902582 | -0.020330932 | 0.040860154 | -0.020294319 | 0.036388698 |

Li d

| Expt-TrueIP | | Expt-FitIP | | ppTDAHF-ab | | ppTDAHF-bb | | ppTDAHF-ave | |
|---|---|---|---|---|---|---|---|---|---|
| Exci-IP | Recal QD | Exci-IP | Recal QD | Exci-IP | Recal QD | Exci-IP | Recal QD | Exci-IP | Recal QD |
| -0.05559856 | 0.001160449 | -0.055607806 | 0.001409765 | -0.055591824 | 0.000978776 | -0.055593002 | 0.00101055 | -0.055592424 | 0.000994943 |
| -0.031265117 | 0.000967105 | -0.031274362 | 0.001558276 | -0.031277964 | 0.001788513 | -0.031278452 | 0.001819703 | -0.031278219 | 0.00180477 |
| -0.020003338 | 0.000417166 | -0.020012584 | 0.001572201 | -0.020022994 | 0.002871807 | -0.020023092 | 0.002884036 | -0.020023054 | 0.002879215 |
| -0.013886689 | -0.000475135 | -0.013895935 | 0.001521436 | -0.013904404 | 0.003348516 | -0.013904292 | 0.003324365 | -0.013904359 | 0.003338676 |

IV. QD fit results

| | Allext | | | Exp-fit | | | ppTDAHF | | |
|---|---|---|---|---|---|---|---|---|---|
| | a | b | c | a | b | c | a | b | c |
| Be 1S | 0.671066791 | -0.140129233 | 0.330008452 | 0.673697493 | -0.065681334 | 0.840771055 | 0.671937593 | -0.091213721 | 0.661433857 |
| 3S | 0.772336813 | -0.47278779 | -0.114336894 | 0.777691183 | -0.332651501 | 0.755653801 | 0.773154284 | -0.385302533 | 0.444876929 |
| 1P | 0.366977664 | 0.794641709 | -3.74837204 | 0.365634153 | 0.769150162 | -3.862470435 | 0.331954103 | 0.268195143 | -6.935389666 |
| 3P | 0.360162937 | -0.479703979 | 1.488226604 | 0.369980733 | -0.322718023 | 1.971050676 | 0.3642613 | -0.344117672 | 1.939938959 |
| 1D | -0.101748269 | 0.334041432 | -31.29063078 | -0.104394865 | 0.215194848 | -32.70534209 | -0.12536165 | 1.626712594 | -12.65892334 |
| 3P | 0.104134554 | -0.213076121 | -2.020507328 | 0.11601708 | 0.253848762 | 2.683768561 | | | |

0.083484581 0.229735263 0.427242402
Mg 1S 1.519666606 -0.214951556 0.685549079 1.522202626 -0.136381133 1.284741362
1.519299353 0.086798193 3.069110765
3S 1.624069034 -0.650383779 -0.001525729 1.626378336 -0.584225655 0.455208342
1.621127666 -0.400299919 1.869591748
1P 1.045571532 0.450877921 -1.449620028 1.047319706 0.490832623 -1.233049265
1.0446673 0.676270305 -0.946567224
3P 1.125386475 -0.770313508 2.271503154 1.126868647 -0.741865458 2.384171216
1.125084416 -0.707059164 2.628869977
1D 0.603040735 5.849415064 25.35901556 0.605824914 5.942135209 26.15844573
0.599422926 3.837058757 -1.562675219
3D 0.165548302 -0.109294449 -0.356906242 0.168822511 0.015359506 0.853808406
0.13841276 0.420455096 2.006201332

Allext Exp-fit
ppTDAHFAB ppTDAHFBB ppTDAHFAVE

a b c a b c
a b c a b c a
b c
Li 2S 0.39620515 -0.167641433 -0.899477236 0.399067115 -0.071852628 -0.097465032
0.421514577 0.142922337 1.699147316 0.392520339 0.147934722 1.759963637 0.407050636
0.143725656 1.722922532
2P 0.045294073 0.004577127 -0.24254609 0.047040613 0.043335083 -0.043487673
0.033260307 0.062381149 0.076901206 0.042311207 0.066836413 0.060215892 0.037791277
0.064518527 0.068152751
2D -0.002349623 -0.167757542 -1.885429226 0.001411789 -0.011353166 -0.205156952
0.005223744 0.148751448 1.299887377 0.005124866 0.141974113 1.22009066 0.00517852
0.145537914 1.261869398

V. QD fit parabola results

| Be | True IP | | | Fit IP | | | ppTDA | | | ALDA | | |
|---|---|---|---|---|---|---|---|---|---|---|---|---|
| | a | dmu | d2mu | a | dmu | d2mu | a | dmu | d2mu | a | dmu | d2mu |
| 1S | 0.671 | -0.016 | 0.001 | 0.674 | -0.013 | 0.002 | 0.672 | -0.014 | 0.001 | 0.654 | -0.028 | 0.000 |
| 3S | 0.772 | -0.049 | 0.000 | 0.778 | -0.043 | 0.002 | 0.773 | -0.045 | 0.001 | 0.771 | -0.041 | 0.000 |
| 1P | 0.367 | 0.201 | -0.021 | 0.366 | 0.200 | -0.021 | 0.332 | 0.186 | -0.037 | 0.333 | 0.124 | -0.082 |
| 3P | 0.360 | -0.204 | 0.022 | 0.370 | -0.194 | 0.029 | 0.364 | -0.196 | 0.028 | 0.415 | 0.090 | 0.000 |
| 1D | -0.102 | 0.092 | -0.019 | -0.104 | 0.089 | -0.020 | -0.125 | 0.107 | -0.007 | 0.173 | -0.050 | 0.021 |

| | | | | | | | | | | | | |
|---|---|---|---|---|---|---|---|---|---|---|---|---|
| 3D | 0.104 | -0.006 | -0.002 | 0.116 | 0.006 | 0.002 | 0.083 | 0.012 | 0.000 | 0.174 | 0.004 | 0.002 |

| Mg | True IP | | | Fit IP | | | ppTDA | | |
|---|---|---|---|---|---|---|---|---|---|
| | a | dmu | d2mu | a | dmu | d2mu | a | dmu | d2mu |
| 1S | 1.520 | -0.022 | 0.001 | 1.522 | -0.020 | 0.002 | 1.519 | -0.014 | 0.005 |
| 3S | 1.624 | -0.061 | 0.000 | 1.626 | -0.058 | 0.001 | 1.621 | -0.053 | 0.004 |
| 1P | 1.046 | 0.076 | -0.005 | 1.047 | 0.078 | -0.005 | 1.045 | 0.094 | -0.003 |
| 3P | 1.125 | -0.215 | 0.019 | 1.127 | -0.213 | 0.020 | 1.125 | -0.215 | 0.022 |
| 1D | 0.603 | 0.284 | 0.031 | 0.606 | 0.287 | 0.032 | 0.599 | 0.276 | -0.002 |
| 3D | 0.166 | -0.005 | 0.000 | 0.169 | -0.002 | 0.001 | 0.138 | 0.018 | 0.002 |

| Li | True IP | | | Fit IP | | | AB | | | BB | | | AVE | | |
|---|---|---|---|---|---|---|---|---|---|---|---|---|---|---|---|
| | a | dmu | d2mu | a | dmu | d2mu | a | dmu | d2mu | a | dmu | d2mu | a | dmu | d2mu |
| S | 0.396 | -0.007 | -0.001 | 0.399 | -0.005 | 0.000 | 0.422 | 0.001 | 0.002 | 0.393 | 0.001 | 0.002 | 0.407 | 0.001 | 0.002 |
| P | 0.045 | 0.005 | -0.001 | 0.047 | 0.006 | 0.000 | 0.033 | 0.007 | 0.000 | 0.042 | 0.008 | 0.000 | 0.038 | 0.007 | 0.000 |
| D | -0.002 | -0.003 | -0.001 | 0.001 | 0.000 | 0.000 | 0.005 | 0.004 | 0.001 | 0.005 | 0.004 | 0.001 | 0.005 | 0.004 | 0.001 |

VI. Excitation Energy extrapolation for Be 1P series through QD fitting

| | Expt | pp-TDA | ALDA |
|---|---|---|---|
| 2p | 0.1939 | 0.1959 | 0.1868 |
| 3p | 0.2743 | 0.2737 | 0.271 |
| 4p | 0.3054 | 0.3047 | 0.3048 |

| | | | |
|---|---|---|---|
| 5p | 0.3195 | 0.3186 | 0.3194 |
| 6p | 0.3269 | 0.3259 | 0.3269 |
| 7p | 0.3313 | 0.3302 | 0.3313 |
| 8p | 0.334 | 0.3329 | 0.3341 |
| 9p | 0.3359 | 0.3348 | 0.3359 |
| 10p | 0.3372 | 0.3361 | 0.3372 |
| 11p | 0.3382 | 0.337 | 0.3382 |
| 12p | 0.3389 | 0.3378 | 0.3389 |

Note: In the main article, all Expt data reported are real ones, not these fitted/extrapolated results, the 2p-5p data for pp-TDA are from calculation while 6p-12p are above extrapolated results, the 2p-4p data for ALDA are calculated while 5p-12p are above extrapolated results.
